# Supplementary material for: Subquadratic Multivalued Asynchronous Byzantine Agreement WHP
Source: arXiv:2308.02927 source file (2023-08-05)
Supplement: Supplementary file 1 [file approver_appendix.tex]

\section{Approver proofs}
\label{approver_appendix}

\approvervalidity*
\begin{proof}
By Claim \ref{sampling} S4 holds whp for the four sampled committees. It remains to show that S4 implies validity. Since by S4 the number of Byzantine processes sampled to the init committee in line \ref{l.app.comm1} is at most $B$, no process receives $B+1$ messages with a value $w\neq v$. Thus, no correct process echoes $\lr{\textsc{echo},w}$ in line \ref{l.app.comm2_and_echo}. 
Because the number of Byzantine processes in $C(\lr{\textsc{echo},w},\lambda)$ in line \ref{l.app.comm2_and_echo} is also at most $B$, no correct process receives more than $B$ $\lr{\textsc{echo},w}$ messages.
As a result, since $B<W$, no $\lr{\textsc{ok},w}$ message is sent by any correct process.
Since ok messages carry proofs, no Byzantine process can send a valid $\lr{\textsc{ok},w}$ either. Therefore, the only possible value in the ok messages is $v$, and no other value is returned.
\end{proof}

\approveragreement*

\begin{proof}

By Claim \ref{sampling} and Corollary \ref{S5}, S4 and S5 hold whp for the four sampled committees. We show that S4 and S5 imply graded agreement.
Assume $p_i$ returns $\{v\}$ and $p_j$ returns $\{w\}$. Then $p_i$ receives $W$ $\lr{\textsc{ok},v}$ messages and $p_j$ receives $W$ $\lr{\textsc{ok},w}$ messages. 
By S5, two sets of size $W$ intersect by at least $(\frac{1}{3}-d)\lambda+1$ processes. Hence, since by S4 there are at most $B$ Byzantine processes in the ok committee, there is at least one correct process $p_k$ whose ok message is received by both $p_i$ and $p_j$ whp. It follows that $p_k$ sends $\lr{\textsc{ok},v}$ and $\lr{\textsc{ok},w}$. Since every correct process sends at most one ok message (line \ref{l.app.comm3}), $v=w$.
\end{proof}

\approvertermination*
\begin{proof}
By Claim \ref{sampling} S3 holds whp. We show that S3 implies termination. Because all correct processes invoke approve, every correct init committee member in line \ref{l.app.comm1} sends $\lr{\textsc{init},v_i}$.
Notice that $\frac{1}{2}W > (\frac{1}{3}-d)\lambda \geq B$. Hence, since the number of correct processes in the init committee is at least $W$ (S3) and correct processes may send at most two different initial values (Assumption \ref{two_values}), one of them is sent by at least $B+1$ correct processes.
Denote this value by $v$.
Every correct process receives this value from $B+1$ processes, and if it is sampled to $C(\lr{\textsc{echo},v},\lambda)$ in line \ref{l.app.comm2_and_echo} then it sends it to all other processes. 
Since $C(\lr{\textsc{echo},v},\lambda)$ also has at least $W$ correct processes (S3), every correct process $p$ receives $W$ $\lr{\textsc{echo},v}$ messages.
If $p$ is sampled to the ok committee in line \ref{l.app.comm3} and at this point $p$ has not yet sent an $\lr{\textsc{ok},*}$ message, it sends one.
Since there are at least $W$ correct processes that are sampled to the ok committee (S3) and they all send $\textsc{ok}$ messages (possibly for different values), every correct process receives $W$ $\textsc{ok}$ messages and returns the non-empty set of approved values.

\end{proof}
