# Supplementary material for: Subquadratic Multivalued Asynchronous Byzantine Agreement WHP
Source: arXiv:2308.02927 source file (2023-08-05)
Supplement: Supplementary file 2 [file whp_coin_appendix.tex]

\section{WHP Coin Proofs}
\label{whp_coin_appendix}

In the committee-based protocol, a value $v$ is \emph{common} if at least $B+1$ correct processes in $C(\textsc{second},\lambda)$ have $v_i=v$ at the end of phase 1. The next lemma adapts the lower bound of Lemma \ref{common_vals} on the number of common values to the committee-based protocol.
 
% \begin{restatable}{lemma}{recommon}
\begin{lemma}
\label{common_vals_comm}
In Algorithm \ref{alg:shared_coin_comm_protocol} whp, $c \geq \frac{d(11-3d)}{1+9d}\lambda$.
\end{lemma}
% \end{restatable}
% \recommon*

\begin{proof}

Let $n_1=|C(\textsc{first},\lambda)|,n_2=|C(\textsc{second},\lambda)|$.
We define a table T with $n_2$ rows and $n_1$ columns. 
For each correct process $p_i\in C(\textsc{second},\lambda)$ and each $0\leq j\leq n_1-1$, $T[i,j]=1$ iff $p_i$ receives $\lr{\textsc{first},v}$ from $p_j\in P_1$ before sending the \textsc{second} message in line \ref{l.com.send_second}.
Each row of a correct process contains exactly
$W$ ones since it waits for $W$ $\lr{\textsc{first},v}$ messages (line \ref{l.com.wait_first}). Each row of a faulty process in $C(\textsc{second},\lambda)$ is arbitrarily filled with $W$ ones and $n_1-W$ zeros.
Thus the total number of ones in the table is $n_2W$ and the total number of zeros is $n_2(n_1-W)$.
Let $k$ be the number of columns with at least $2B+1$ ones.
Each column represents a value sent by a process in $C(\textsc{first},\lambda)$.
By S4, whp, at most $B$ of the processes that receive this value are Byzantine.
Thus, whp, out of any $2B+1$ ones in each of these columns, at least $B+1$ represent correct processes that receive this value and it follows that $c\geq k$.

Denote by $x$ the number of ones in the remaining columns. Because each column has at most $n_2$ ones we get:

\begin{equation}
x \geq n_2W-kn_2 =
n_2 \left \lceil{(\frac{2}{3}+3d)\lambda}\right \rceil -kn_2
\geq n_2(\frac{2}{3}+3d)\lambda-kn_2.
\end{equation}

And because the remaining columns have at most $2B$ ones:
\begin{equation}
x \leq 2B(n_1-k)
= 2\left \lfloor{(\frac{1}{3}-d)\lambda}\right \rfloor(n_1-k)
\leq 2(\frac{1}{3}-d)\lambda(n_1-k).
\end{equation}

Combining $(1),(2)$ we get:

\begin{equation*}
2(\frac{1}{3}-d)\lambda(n_1-k) \geq
n_2(\frac{2}{3}+3d)\lambda-kn_2
\end{equation*}

\begin{equation*}
kn_2-2\lambda k(\frac{1}{3}-d) \geq
n_2(\frac{2}{3}+3d)\lambda-2(\frac{1}{3}-d)\lambda n_1
\end{equation*}

\begin{equation*}
k(n_2-2\lambda (\frac{1}{3}-d)) \geq \lambda(
n_2(\frac{2}{3}+3d)-2(\frac{1}{3}-d)n_1)
\end{equation*}

\begin{equation*}
k \geq \frac{\lambda(
n_2(\frac{2}{3}+3d)-2(\frac{1}{3}-d)n_1)}{n_2-2\lambda (\frac{1}{3}-d)}
\end{equation*}

By S2 for $C(\textsc{second},\lambda)$, whp $n_2\geq(1-d)\lambda$ and we get:

\begin{equation*}
k \geq \frac{\lambda(
(1-d)\lambda(\frac{2}{3}+3d)-2(\frac{1}{3}-d)n_1)}{n_2-2\lambda (\frac{1}{3}-d)}
\end{equation*}

By S1 for $C(\textsc{first},\lambda)$ and $C(\textsc{second},\lambda)$, whp $n_1,n_2\leq (1+d)\lambda$ and we get:

\begin{equation*}
k \geq \frac{\lambda \bigg[
(1-d)\lambda(\frac{2}{3}+3d)-2(\frac{1}{3}-d)(1+d)\lambda \bigg]}{(1+d)\lambda-2\lambda (\frac{1}{3}-d)}=\frac{\lambda\bigg[
(1-d)(\frac{2}{3}+3d)-2(\frac{1}{3}-d)(1+d)\bigg]}{(1+d)-2 (\frac{1}{3}-d)}
\end{equation*}

Finally, we get whp:

\begin{equation*}
c \geq k \geq \frac{d(11-3d)}{1+9d}\lambda.
\end{equation*}
as required.

\end{proof}

Let $v_{min}\triangleq \displaystyle \min_{ p_i \in C(\textsc{first},\lambda)}\{VRF_i(r)\}$. Similiarly to Lemma \ref{common_prob}, we prove that the probability that it is common is bounded by a constant, whp. I.e., we show that $Prob[v_{min}\;is\;common]\geq const\cdot g(n)$ where $g(n)$ goes to $1$ as $n$ goes to infinity.

% \begin{restatable}{lemma}{recommonprob}
\begin{lemma}
\label{common_prob_comm}
whp $Prob[v_{min}\;is\;common]\geq \frac{2}{3(1-d)}\cdot \frac{c-B}{(1+d)\lambda-B}$.
\end{lemma}
% \end{restatable}
% \recommonprob*

\begin{proof}

Notice that we assume that the invocation of whp\textunderscore coin$(r)$ by every process is causally independent of its progress at other processes. Hence, for any two processes $p_i, p_j\in C(\textsc{first},\lambda)$, the messages $\lr{\textsc{first},v_i}$, $\lr{\textsc{first},v_j}$ are causally concurrent.
Thus, due to our \emph{delayed-adaptive adversary} definition,
these messages are scheduled by the adversary regardless of their content, namely their VRF random values.
Notice that the adversary can corrupt processes before they initially send their VRF values.
By S4 there are at most $B$ Byzantine processes in $C(\textsc{first},\lambda)$. 
Since the adversary cannot predict the VRF outputs, the probability for a given process to be corrupted before sending its \textsc{first} messages is at most $\frac{B}{|C(\textsc{first},\lambda)|}$.
The adversary is oblivious to the correct processes' VRF values when it schedules their first phase messages. Therefore, each of them has the same probability to become common. Since at most $B$ common values are from Byzantine processes, this probability is at least $\frac{c-B}{|C(\textsc{first},\lambda)|-B}$.
 We conclude that $v_{min}$ is common with probability at least $(1-\frac{B}{|C(\textsc{first},\lambda)|})\frac{c-B}{|C(\textsc{first},\lambda)|-B}$.
By S1 and S2 we get that $(1-d)\lambda \leq |C(\textsc{first},\lambda)| \leq (1+d)\lambda$ whp.

Thus, whp, $v_{min}$ is common with probability at least $(1-\frac{B}{(1-d)\lambda})\frac{c-B}{(1+d)\lambda-B}=
(1-\frac{\left \lfloor{(\frac{1}{3}-d)\lambda}\right \rfloor}{(1-d)\lambda})\frac{c-B}{(1+d)\lambda-B} \geq
(1-\frac{(\frac{1}{3}-d)\lambda}{(1-d)\lambda})\frac{c-B}{(1+d)\lambda-B}=
\frac{2}{3(1-d)}\cdot \frac{c-B}{(1+d)\lambda-B}
$.

\end{proof}

\begin{lemma}
\label{common_global_min_comm}
If $v_{min}$ is common then whp each correct process holds $v_{min}$ at the end of phase 2.
\end{lemma}
\begin{proof}
Since $v_{min}$ is common, at least $B+1$ correct members of $C(\textsc{second},\lambda)$ receive it by the end of phase 1 and update their local values to $v_{min}$. During the second phase, each correct process hears from $W$ members of $C(\textsc{second},\lambda)$ whp. By S6, this means that it hears from at least one correct process that has updated its value to $v_{min}$ and sent it whp.
\end{proof}

\begin{lemma}
\label{safety_comm}
Let $\rho=\frac{18d^2+27d-1}{3(5+6d)(1-d)(1+9d)}$. Algorithm \ref{alg:shared_coin_comm_protocol} implements a shared coin with success rate $\rho$, whp.
\end{lemma}

\begin{proof}
Denote $n_1=|C(\textsc{first},\lambda)|$. We bound whp the probability that all correct processes output $b\in \{0,1\}$ as follows:

 $Prob[$all correct processes output $b]\geq
 Prob[$all\;correct\;processes\;have\;the\;same\;$v_i$ at the end of phase 2\;and\;its\;LSB\;is\;$b]\geq Prob[$all\;correct\;processes have $v_i=v_{min}$  at the end of phase 2 and its LSB is $b]=\frac{1}{2} \cdot Prob[$all\;correct\;processes have $v_i=v_{min}]\stackrel{\text{Lemma \ref{common_global_min_comm}}}{\geq}
 \frac{1}{2} \cdot Prob[v_{min}$ is common$]\stackrel{\text{Lemma \ref{common_prob_comm}}}{\geq} \frac{1}{2} \cdot \frac{2}{3(1-d)}\cdot \frac{c-B}{(1+d)\lambda-B} \stackrel{\text{Lemma \ref{common_vals_comm}}}{\geq}
 \frac{1}{3(1-d)}\cdot \frac{\frac{d(11-3d)}{1+9d}\lambda-B}{(1+d)\lambda-B} =
 \frac{1}{3(1-d)}\cdot \frac{\frac{d(11-3d)}{1+9d}\lambda-\left \lfloor{(\frac{1}{3}-d)\lambda}\right \rfloor}{(1+d)\lambda-\left \lfloor{(\frac{1}{3}-d)\lambda}\right \rfloor} \geq
 \frac{1}{3(1-d)}\cdot \frac{\frac{d(11-3d)}{1+9d}\lambda-(\frac{1}{3}-d)\lambda}{(1+d)\lambda-((\frac{1}{3}-d)\lambda-1)}=
 \frac{1}{3(1-d)}\cdot \frac{\lambda\frac{18d^2+27d-1}{27d+3}}{\lambda(\frac{2}{3}+2d)+1}\geq
 \frac{1}{3(1-d)}\cdot \frac{\lambda\frac{18d^2+27d-1}{27d+3}}{\lambda(\frac{2}{3}+2d)+\lambda}=
\frac{18d^2+27d-1}{3(5+6d)(1-d)(1+9d)}$.
 
\end{proof}

We have shown a bound on the coin's success rate whp. Since $d>0.0362$, the coin's success rate is a positive constant whp.
We next prove that the coin ensures liveness whp.
 
\begin{lemma}
\label{shared_coin_termination_comm}
If all correct processes invoke Algorithm \ref{alg:shared_coin_comm_protocol} then all correct processes return whp.
\end{lemma}

\begin{proof}
All correct processes in $C(\textsc{first},\lambda)$ send their message in the first phase.
At least $W$ of them are correct whp by S3. All correct processes in $C(\textsc{second},\lambda)$ eventually receive $W$ $\lr{\textsc{first},x}$ messages whp and send a message in the second phase. As ,whp, again $W$ correct processes send their messages (by S3), each correct process eventually receives $W$ $\lr{\textsc{second},x}$ messages and returns whp.
\end{proof}

From Lemma \ref{safety_comm} and Lemma \ref{shared_coin_termination_comm} we conclude:

\rewhpcoin*
